# Supplementary material for: Classical-to-Topological Transmission Line Couplers
Source: arXiv:2104.01162 ancillary file (2021-03-11)
Supplement: Supplementary file 1 [file CouplerPaper_Supplemental.pdf]

# Supplementary Materials for Classical-to-Topological Transmission Line Couplers

Robert J. Davis,[1,*] Dia'aaldin J. Bisharat,[1,2] and Daniel F. Sievenpiper[1]

[1]*Electrical Engineering Department, University of California, La Jolla, California 92093, USA*
[2]*Photonics Initiative, Advanced Science Research Center, City University of New York, New York, New York 10031, USA*

(Dated: February 26, 2021)

## I. FIELD DECAY AND FINITE EFFECTS OF VARIOUS BULK SIZES

The model analyzed in the main text employs only 3 unit cells on either side of the interface mode. This may seem surprising, considering the overall approximation being made is of the infinite bulk used to derive the topological behavior of the band structure, but it is well supported by considering the practical effects of the system. Physically, the metallic elements present a very high contrast for the photonic crystal-like structure, which implies a rapid decay into the bulk [1].

To see this, Fig. 1 shows the simulated magnitude of the electric field 0.1 mm above the surface of a 10-cell long and variable width sample, excited via a wave port on the bottom of the plot. Fig. 1(a) shows the fields with a bulk size of 10 unit cells on either side of the interface (20 total), while Fig. 1(b) shows the fields using only 3 cells on either side. They appear visually identical. However, if we then consider fewer bulk cells, the situation changes. Fig. 1(c) shows a 2-cell bulk, and Fig. 1(d) shows a single cell bulk. The 2-cell case appears to still work, but there is now a visual difference appearing along the outer edges of the sample. As expected, the single cell case hardly works at all, with considerable field concentration at the transition region between the antipodal feed and the interface. The mode that is propagating here is no longer topological, but rather closer to a modified form of antipodal twin line, which has large scattering at each zig-zag bend.

For a more quantitative verification, we can also observe the scattering parameters as a function of bulk width. Fig. 2(a) shows $S_{11}$ and $S_{21}$ of the results of Fig. 1. As expected, we see that there is essentially no difference in insertion loss for more than 3 unit cells, and negligible difference in return losses. Likewise, we see a rapid decrease below 3 cells.

A general way of characterizing this from a fields perspective (without needing to know the S parameters) is given in Fig. 2(b), where we plot the estimated minimum number of cells required to contain 90% of the total fields in the plane of propagation as a function of the total number of unit cells simulated. This is determined by integrating the fields along a line $l$ stretching from the interface outwards laterally as a function of distance $x$, and taking the first point where the the value is greater than or equal to the threshold $\tau$,

$$Cf(l) \equiv \frac{\int_{l_{min}}^{l} |E(x)|^2 dx}{\int_{l_{min}}^{l_{max}} |E(x)|^2 dx} \geq \tau. \qquad (1)$$

When $Cf(l) > 0.9$, 90% of the total fields are therefore contained within the distance, the result of which is given in Fig. 2(b). The dashed line is simply the value when the number of cells required is equal to the number simulated, which we see is first reached when three cells are included. For this case the line of integration is placed in the middle of the sample (5 unit cells in) at the $0.25a$ point of the cell, and at the zero point between the two complementary layers, stretching out from the interface to the right hand side. By symmetry the result is the same if we flip it to the left hand side as well. Note that this last analysis is easily applicable to other interface-mode systems as well.

* Authors to whom correspondence should be addressed: Robert Davis, rjdavis@ucsd.edu; Daniel Sievenpiper, dsievenpiper@ucsd.edu

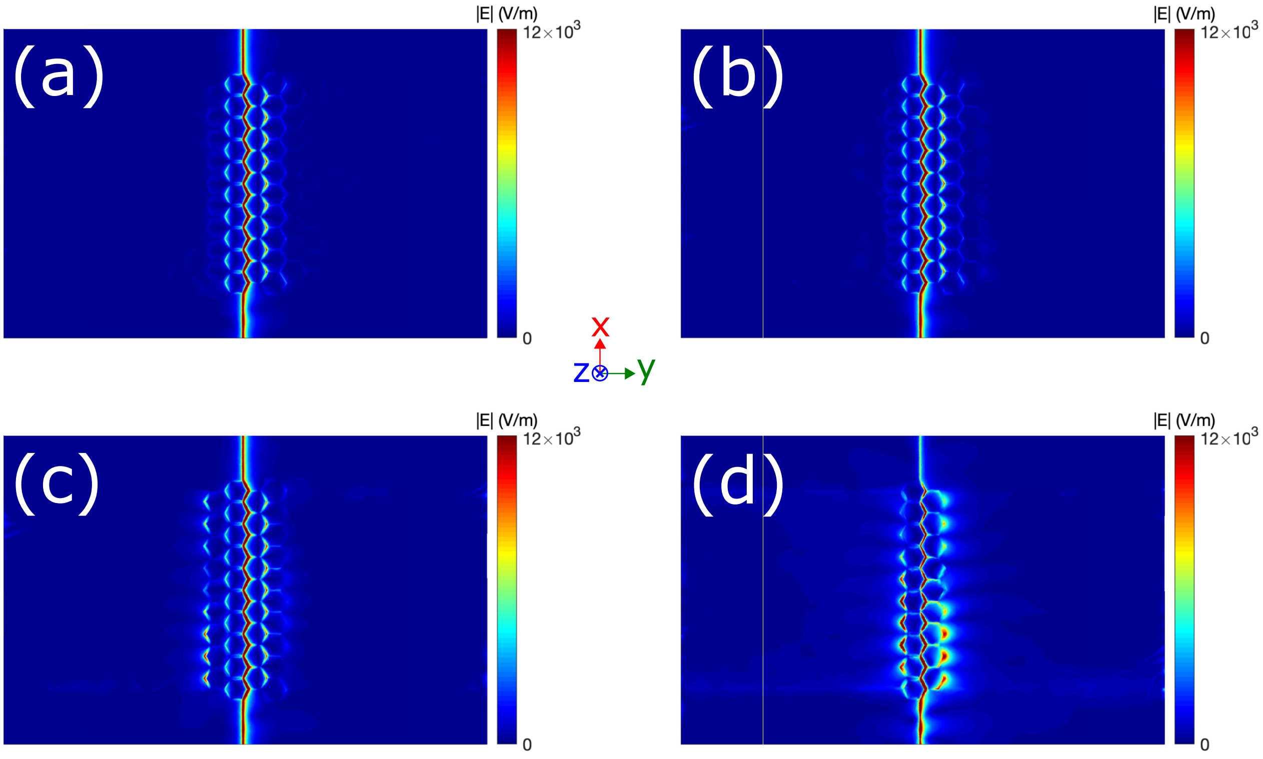


FIG. 1. Simulated electric field effects of finite bulks. Panels (a), (b), (c), and (d) show the magnitude of the electric field 0.1 mm above the top layer of the PTI for a lateral bulk side of 10, 3, 2, and 1 cells on either side of the interface, respectively. Note that there is no visual difference between the 10 and 3 cell case, supporting the choice of using 3 cells. Further, the 2 and 1 cell cases show larger and larger deviations from the "infinite" case, leading to field build up and deterioration of the PTI mode, supporting the lower bound of 3 cells.

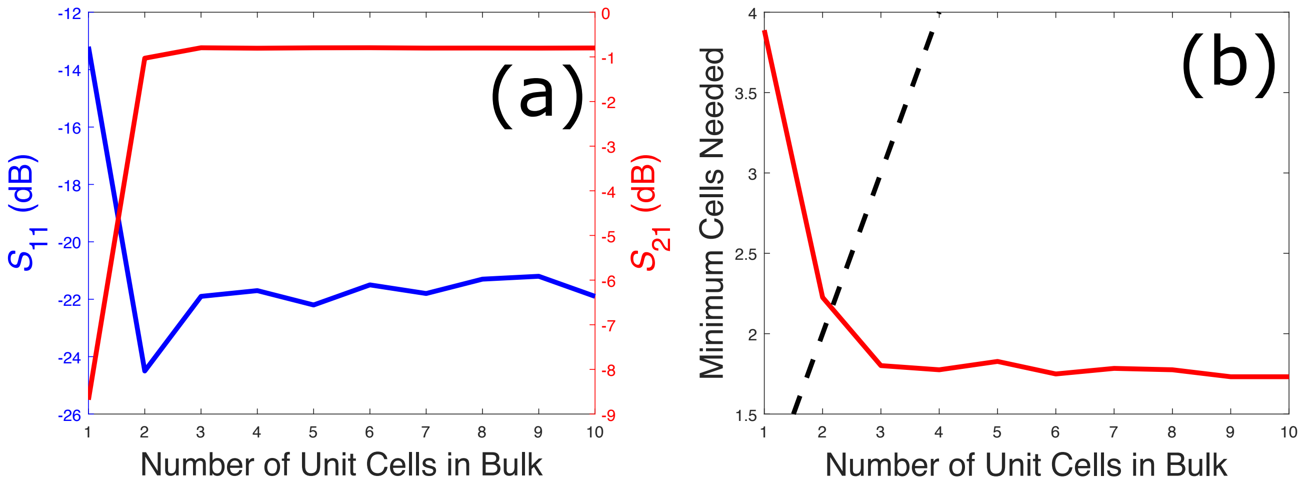


FIG. 2. Quantitative effects of finite bulk width. Panel (a) shows the simulated scattering parameters of the 10-cell long device as a function of the number of lateral bulk cells. We see that there is essentially no transmission for 1 cell, slightly higher transmission for 3 than 2 cells, and negligible change for larger bulks. (b) shows a general description of the required number of cells needed to contain 90% of the E field as a function of the number of cells simulated. The dashed line represents the point where the required cells matches the simulated cells, which we see is satisfied beginning at 3 cells (points below the line).

## II. SHARP TURNS AND MAGIC T FREQUENCY RESPONSES

Fig. 3 presents the full simulated frequency response of the "torturous path" sharp turning model presented in the main text, which includes all forms of loss. It can be seen that the behavior closely matches the straight path case of the main text, with the overall reduction in transmission coming primarily as a result of the extra propagation length, rather than scattering from the sharp turns. This is one of the attractive features of PTI-based designs, for the symmetries of their system cause there to be essentially zero coupling between forward and backward propagating modes.

Likewise, Fig. 4 presents the simulated frequency response of the "Magic T" presented in the main text, broken down into the four different active channel configurations. Part (a), (b), (c), and (d) show the relevant S parameters for an excitation for ports 1, 2, 3, and 4, respectively. In each case we can observe that 1. the reflection is below -10 dB for the full bandwidth of the device, 2. the "forward" channel, which is the direction that requires a spin-flip process to couple and is therefore expected to be very small, is indeed below -20 dB for most of the bandwidth, 3. side channel 1 is above -2 dB for most of the bandwidth, much the same as a straight configuration, and 4. side channel 2, which is across the symmetry gap, is around -10 dB for most of the bandwidth. As discussed in the text, the lack of symmetry right at the junction between the two channels caused by the triangular lattice results the difference between the two side channels. Nevertheless, the "forbidden" forward channel is still more than -10 dB lower than the lowest of the two side channels, proving substantial isolation even in the most basic case.

[1] J. Joannopoulos, S. G. Johnson, J. N. Winn, and D. M. Robert, *Photonic Crystals: Molding the Flow of Light* (Princeton University Press, 2008).

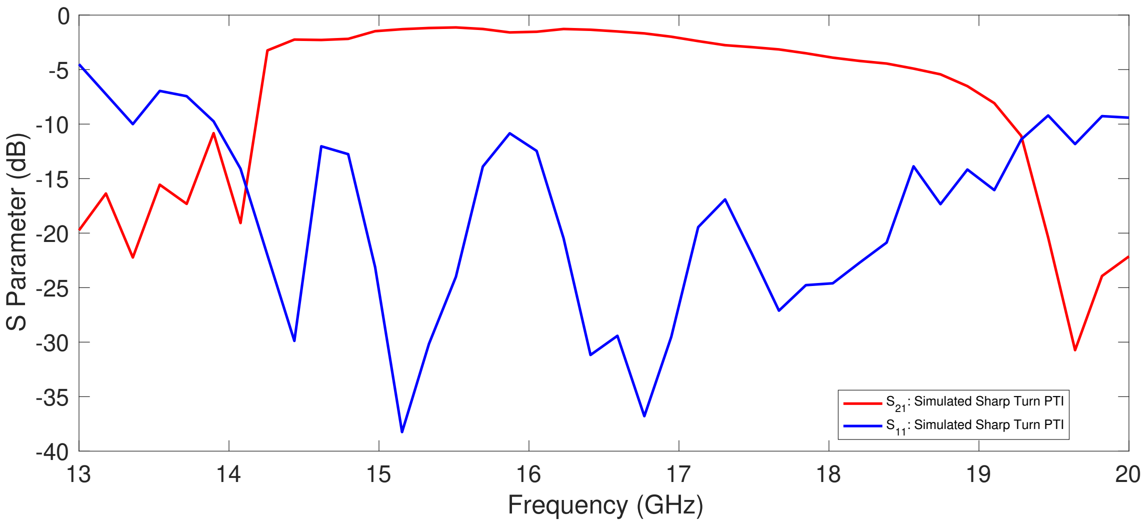


FIG. 3. Frequency response of the 2-turn "torturous path" sharp turn simulation. All losses are included. Note that the behavior is nearly identical to the straight path, with the decrease in $S_{21}$ caused primarily by the extra propagation losses.

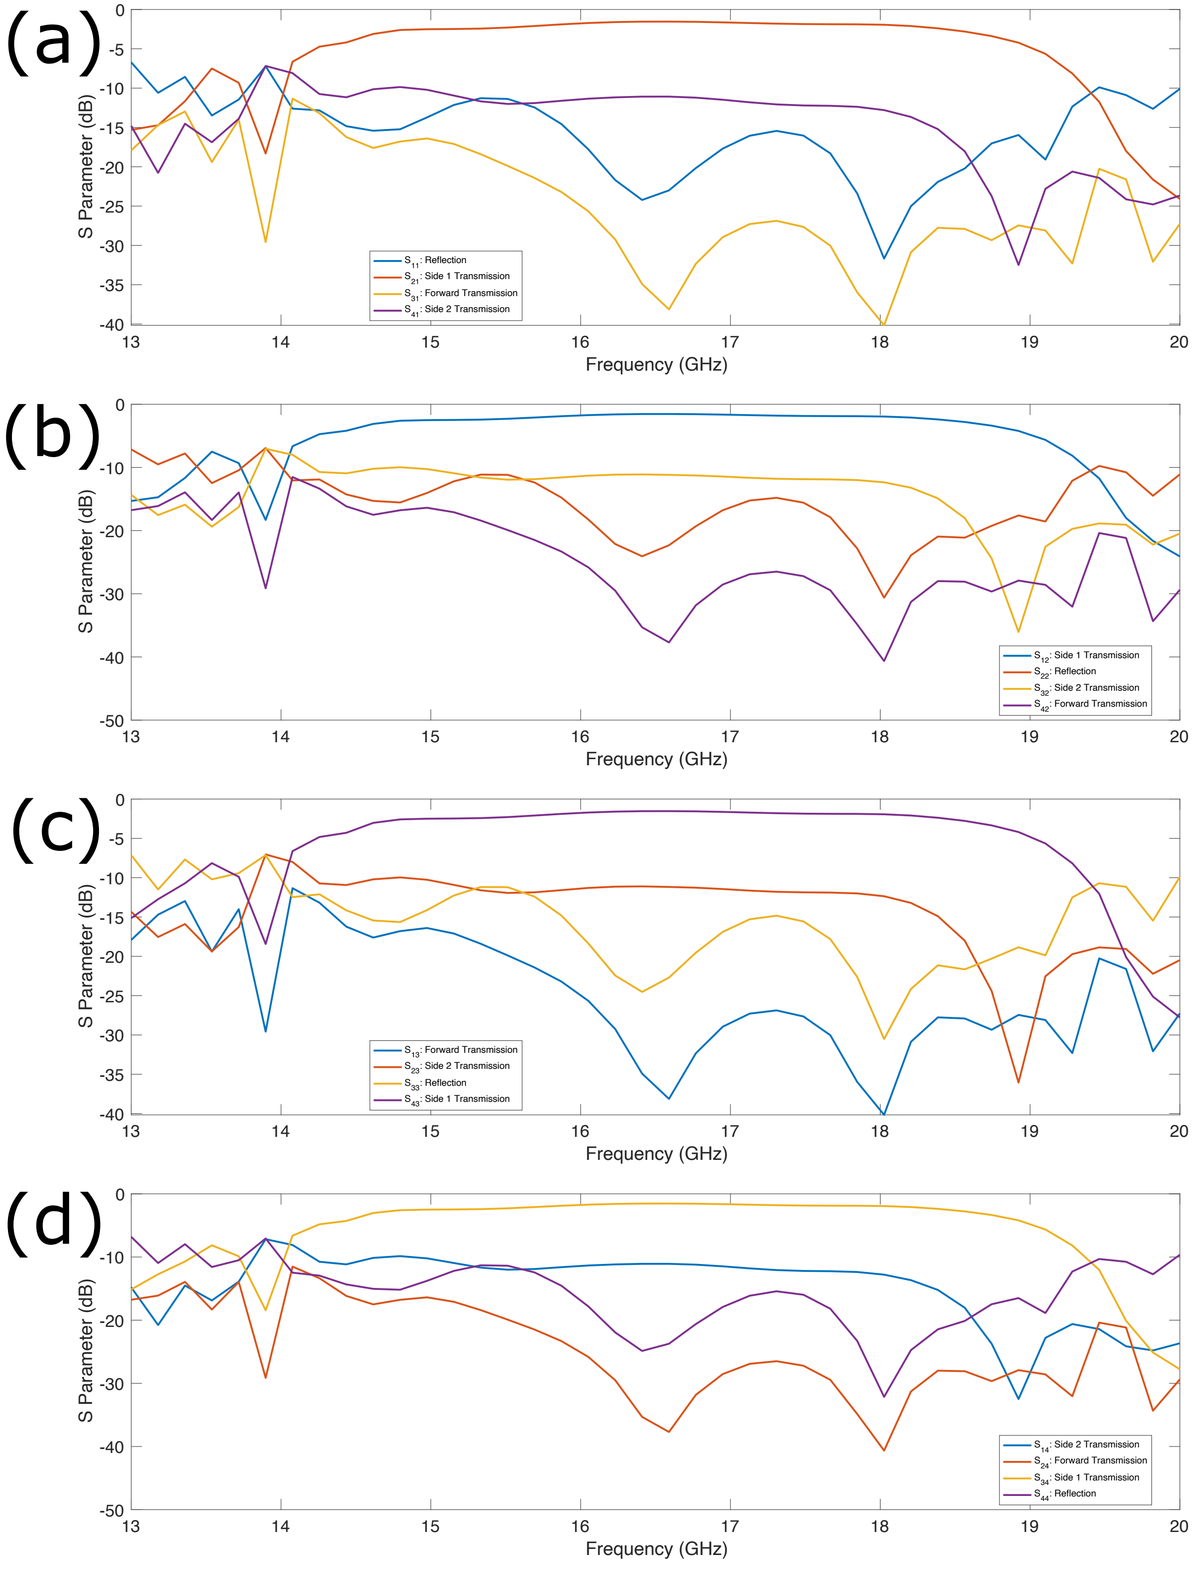


FIG. 4. Frequency response of the simulated magic T presented in the main text. (a): Port 1 excited, (b): Port 2 excited, (c): Port 3 excited, (d): Port 4 excited. As expected, all four situations result in identical behavior, with the "forbidden" forward channel being as low as -30 dB, the lowest side channel (across the gap) being close to -10 dB, and the highest side channel being above -2 dB.
